# Supplementary material for: Identifying the Mechanism of Continued Growth of the Solid-Electrolyte Interphase
Source: arXiv:1812.03841 ancillary file (2018-12-11)
Supplement: Supplementary file 1 [file appendix.pdf]

# Supporting Information: Identifying the Mechanism of Continued Growth of the Solid-Electrolyte Interphase

Fabian Single and Birger Horstmann*

*German Aerospace Center (DLR), Institute of Engineering Thermodynamics, Pfaffenwaldring 38-40, 70569 Stuttgart, Germany and Helmholtz Institute Ulm (HIU), Helmholtzstraße 11, 89081 Ulm, Germany*

Arnulf Latz

*German Aerospace Center (DLR), Institute of Engineering Thermodynamics, Pfaffenwaldring 38-40, 70569 Stuttgart, Germany Helmholtz Institute Ulm (HIU), Helmholtzstraße 11, 89081 Ulm, Germany and Ulm University, Institute of Electrochemistry, Albert-Einstein-Allee 47, 89069 Ulm, Germany*

(Dated: 11 January 2018)

## 1. SEI GROWTH MODELS

Below we refer to the three LTGMs as $(i) = \mathrm{S}$ (solvent diffusion), $\mathrm{e}^-$ (electron conduction) and $\mathrm{Li_I}$ (lithium interstitial diffusion). We assume that capacity fade consists of two distinct contributions, $Q_{\mathrm{irr}} = Q_{\mathrm{irr}}^{\mathrm{SEI}} + Q_{\mathrm{irr}}^{\mathrm{lin}}$. The former part refers to the irreversible capacity which is trapped inside the SEI and is directly related to the SEI thickness $L$

$$L = \frac{V}{s}\frac{Q_{\mathrm{irr}}^{\mathrm{SEI}}}{AF} + L_0, \tag{SI-1}$$

where $V$ is the mean partial molar volume of the SEI and $s$ is the mean stoichiometric coefficient of species $(i)$ in the SEI formation reaction. $L_0$ is the SEI thickness at the start of the experiment and $A$ is the surface area of the negative electrode. Both $V$ and $s$ are mean quantities because SEI composition is divers. The second part, $Q_{\mathrm{irr}}^{\mathrm{lin}}$, factors in other mechanisms that consume active lithium. These processes are assumed to proceed at a constant rate $\gamma$ which does not depend on the SoC

$$Q_{\mathrm{irr}}^{\mathrm{lin}}(t) = \gamma \cdot t. \tag{SI-2}$$

We assume that the SEI is a homogeneous film which we describe along a model axis perpendicular to the surface of the underlying electrode. It spans from $x = 0$ (electrode/SEI interface) to $x = L$ (SEI/electrolyte interface). Long term SEI growth is facilitated by $j_{\mathrm{SEI}}^{(i)}$, the flux density of SEI precursor $(i)$ in the SEI. It directly increases the amount of lithium consumed by SEI formation

$$\partial_t Q_{\mathrm{irr}}^{\mathrm{SEI}} = \pm A j_{\mathrm{SEI}}^{(i)}. \tag{SI-3}$$

Here, the sign has to be set for each mechanism individually. It is chosen such such that the right hand side of eq. (SI-3) is positive to account for the flux direction and the sign of its charge carriers. The flux densities are given by the well known expressions for diffusion (Fick's law) and conduction (Ohm's law).

$$j_{\mathrm{SEI}}^{\mathrm{S}} = -FD_{\mathrm{EC}} \cdot \nabla c_{\mathrm{EC}} = -FD_{\mathrm{EC}} \cdot \frac{c_{\mathrm{EC},0}}{L}, \tag{SI-4a}$$

$$j_{\mathrm{SEI}}^{\mathrm{e}^-} = -\kappa \cdot \nabla \phi = -\kappa \cdot \frac{\Phi_0 - U}{L}, \tag{SI-4b}$$

$$j_{\mathrm{SEI}}^{\mathrm{Li_I}} = -FD_{\mathrm{Li_I}} \cdot \nabla c_{\mathrm{Li_I}} = FD_{\mathrm{Li_I}} \cdot \frac{c_{\mathrm{Li_I}}}{L}. \tag{SI-4c}$$

Each flux density is the product of a transport parameter ($D_{\mathrm{EC}}$, $\kappa$ and $D_{\mathrm{Li_I}}$) and a driving force which is a gradient. We approximate these gradients with the ratios of the concentration/potential differences between both SEI sides and the SEI thickness $L$. Both, $c_{\mathrm{EC}}$ and $c_{\mathrm{Li_I}}$ are assumed to be zero at the corresponding reaction interface ($x = 0$ for solvent diffusion and $x = L$ for $\mathrm{Li_I}$ diffusion). For electron conduction, the potential is assumed to equal $\Phi_0$ at the reaction interface and $U$ at the electrode/SEI interface, see table SI-2.

Eliminating $L$ in the simplified flux expressions with eq. (SI-1) turns eq. (SI-3) into an ODE for $Q_{\mathrm{irr}}^{\mathrm{SEI}}$. This ODE can be solved analytically if a constant electrode potential $U$ is assumed, see eqs. (6a) to (6d).

We use the model by Li et al.[1] to describe SEI formation caused by electron tunneling. It assumes a thin inner SEI layer, approximately 2 nm thick and a much thicker porous outer layer. Electrons tunnel across the inner layer and reduce electrolyte at the interface, between these layers. We refer to the original article for a full model description.[1] To simulate this LTGM we replace eq. (SI-3) with eq (29) in reference 1. It states a differential equation in "$Q_{SEI}^{st}$" which is equivalent to the variable $Q_{\mathrm{irr}}^{\mathrm{SEI}}$ in our notation.

## 2. SOC DEVELOPMENT

In the experiment, each cell $(j)$ is charged to a unique SoC before the storage period. Below, we refer to this initial SoC as $\mathrm{SoC}_0^{(j)}$. During open circuit storage, the SoC slowly shifts as irreversible reactions consume lithium stored in the anode. Open circuit storage is only interrupted for checkup sequences which are performed periodically in the experiment. They are used to capture the evolution of the cell capacity $Q_{\mathrm{actual}}(t)$. After a checkup sequence, the cells are recharged to their initial SoC, $\mathrm{SoC}_0^{(j)}$. Note that Keil et al. referenced the SoC to the current cell capacity $Q_{\mathrm{actual}}$ for this step in their experiments. We need to consider this because in this modeling work SoC is referenced to $Q_0$, the capacity of the new cell.

As mentioned above, the SoC drift during storage is caused by irreversible reactions

$$\partial_t \mathrm{SoC}^{(j)}(t) = -\partial_t Q_{\mathrm{irr}}^{(j)}(t)/Q_0, \tag{SI-5}$$

where $Q_0$ is the nominal capacity of the new cell. Irreversible reactions also decrease the current cell capacity

$$Q_{\mathrm{actual}}^{(j)}(t) = Q_0 - Q_{\mathrm{irr}}^{(j)}(t). \tag{SI-6}$$

In the experiment, $Q_{\mathrm{actual}}(t)$ is measured in checkup sequences at $t = t_k$. Afterwards the cell is recharged to $\mathrm{SoC}_0^{(j)}$ which is now referenced to $Q_{\mathrm{actual}}(t_k)$ instead of $Q_0$. Using $Q_0$ as a reference, the cells are recharged to

$$\mathrm{SoC}^{(j)}(t_k) = \mathrm{SoC}_0^{(j)} \cdot \left(1 - Q_{\mathrm{irr}}^{(j)}(t_k)/Q_0\right), \tag{SI-7}$$

after the checkup sequence.

To summarize, during open circuit storage eq. (SI-5) is used to describe the continuous evolution of $\mathrm{SoC}^{(j)}$. Equation (SI-7) is used to reset (increase) the SoC after each checkup sequence. Now, both, $Q_{\mathrm{irr}}$ and the SoC can be integrated simultaneously. Such a simulation is shown in fig. 2. Jumps in the SoC and $U$ correspond to the checkup sequences. It can be seen that the anode potential rises by almost 20 mV during the storage experiment. This affects the rate of SEI formation significantly, depending on the LTGM assumed.

## 3. OVERHANG ANODE AREA

The NCR18650PD cells studied in this experiment are designed such that the coated anode area is larger that the coated cathode area (798 $cm^2$ vs 767 $cm^2$).[2] This results in so-called "overhang areas" of the anode. Lithium stored in this part does not participate in regular charge and discharge cycles. However, it can slowly enter/leave the anode during storage and become available for cycling. The driving force for this process is the potential difference between the actual negative electrode and the overhang area. All cells were delivered and stored at approximately 30% SoC before the experiment. We assume this to be the initial SoC of the overhang area. According to the values provided by Keil et al. the overhang area equals 31 $cm^2$ (note that this is an approximation because the coated area mismatch is reduced slightly when the cell is rolled up). This means that the overhang can store up to 4% of the total cell capacity.

The impact of the overhang area on the lithium balance of the cell depends on the SoC the cell is stored at.

- Cells stored at zero SoC feature a large driving force for overhang delithiation (500 mV). Consequently, we expect full delithiation of the overhang area from its initial SoC of 30%. This corresponds to an increase of the cell capacity by 1.2%.

- The anode potential of cells stored between 20-60% SoC is nearly constant because of the first voltage plateau. This means that the driving force for overhang lithiation is small (1-3 mV). Therefore, we expect little to no impact from this effect for cells stored in this SoC range.

- Cells stored at SoCs larger than 60% feature a driving force of approximately 20 mV which is still relatively small. This causes a capacity decrease because the overlap consumes lithium. Note that this process is slow because of the small driving force. Quantifying the corresponding capacity decrease is beyond the scope of this work.

## 4. PARAMETERIZATION

We list the model parameters in tables SI-1 and SI-2.

All LTGMs (apart from solvent diffusion) show little to no SEI formation at high electrode potential or low SoC. Therefore, we want to use the experimentally measured capacity fade of the cell stored at zero SoC to calibrate $Q_{\text{irr}}^{\text{lin}}$ (approximately 3.3% capacity fade in 9.5 months). However, the cell stored at this SoC experiences a capacity increase of 1.2% from the overhang anode area, as calculated above. We consider this in our choice of $\gamma = \partial_t Q_{\text{irr}}^{\text{lin}}$ which is chosen such that $Q_{\text{irr}}^{\text{lin}}$ causes 4.5% capacity fade during 9.5 months of storage.

In our simulations, we use an active electrode surface area of $A = 14.34\,\text{m}^2$ which is 187 times the coated geometric electrode area (767 $\text{cm}^2$). Although SEI has a divers chemistry, we use a single SEI formation reaction to parameterize our simulation. Here, we use formation of lithium ethylene dicarbonate (LiEDC) according to ref. 3

$$2\text{EC} + 2\text{Li}^+ + 2e^- \rightarrow (\text{CHOCO}_2\text{Li}_2)_2 + R\uparrow . \tag{SI-8}$$

The onset potential of SEI formation $\Phi_0$ is chosen as 800 mV vs. Li/Li$^+$which is a common value in literature.[4] We have chosen the lithium interstitial diffusion coefficient $D_{\text{Li}_\text{I}}$ similar to the lithium diffusion coefficient in graphite.[5] Other parameters which determine the throughput of each transport mechanism are listed in table SI-1 ($D_{\text{EC}}$, $A^*$, $\kappa$ and $c_{\text{Li}_\text{I},0}$). $A^*$ is the surface area we use for the electron tunneling model exclusively. These parameters are chosen to fit the curves in fig. 3b and fig. SI-1 to the experimental data. Note that they only scale the amplitude of $Q_{\text{irr}}^{\text{SEI}}(\text{SoC})$ and do not influence the qualitative SoC dependence for all LTGMs except electron tunneling. For the electron tunneling model, most parameters are adopted from the original work, see ref. 1, Table II, 100%. We adjust only two parameters, namely $A$ and $U_2$. The latter is set to $U_2 = E_\text{f}(\text{LiC}_6) - e \cdot \Phi_0$, such that the SEI formation onset potential $\Phi_0$ is equal for all mechanisms.

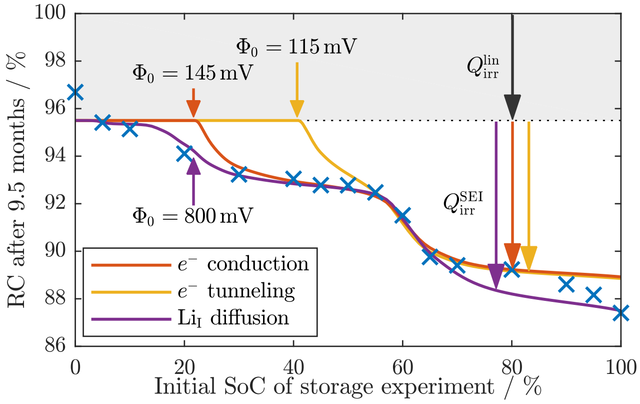


FIG. SI-1. Experimentally obtained relative capacity after 9.5 months of storage (crosses) compared to three different RTLMs (lines). All RTLM characterizing parameters have been chosen for an optimal fit between 50-80% SoC, see table SI-1.

## 5. ALTERNATIVE PARAMETERIZATION

We can improve the qualitative agreement of capacity fade resulting from electron tunneling and electron conduction with the experiment by lowering $\Phi_0$. In this way, we reproduce the characteristic increase of the relative capacity between 55 and 65% SoC, see fig. SI-1. This feature is now reproduced correctly. However, in turn, these mechanisms now predict no SEI formation at low SoCs. Naturally, SEI formation does not take place at SoCs that correspond to an electrode potential that is larger than $\Phi_0$. One could argue that another mechanism could be responsible for the relative capacity change at low SoC. Theoretically, as calculated above, full delithiation of the excess electrode area increases the relative capacity by 1.2%. This increase takes place between zero and 30% initial SoC. However, the measured relative capacity difference between these points equals 3.5%. This means that delithation of the excess electrode area alone cannot explain the experimental data. A second mechanism depending on the SoC is needed to explain this behavior and SEI formation is the only candidate. We conclude that SEI formation is present at low SoCs and low values of $\Phi_0$ are unrealistic.

| | Unit | Figure 3b | Figure SI-1 |
|---|---|---|---|
| $\Phi_0$ | mV vs. $Li/Li^+$ | 800/800/800 | 115/145/800 |
| $\kappa$ | $S\,m^{-1}$ | $8.95{\cdot}10^{-14}$ | $8.20{\cdot}10^{-13}$ |
| $c_{Li_I,0}$ | $mmol\,m^{-3}$ | 15.00 | 15.00 |
| $D_{EC}$ | $m^2\,s^{-1}$ | $2.50{\cdot}10^{-22}$ | - |
| $A^*$ | $m^2$ | 14.34 | 57.37 |

TABLE SI-1: Transport parameters. The three values of the SEI onset potential $\Phi_0$ are given in the following order: electron tunneling/electron conduction/$Li_I$ diffusion. Note that we cannot determine $D_{EC}$,$\kappa$ and $c_{Li_I,0}$ independently of $A$ because they appear as products only.

| | Description | Value | Unit |
|---|---|---|---|
| $U$ | Potential of the negative electrode vs. $Li/Li^+$ | | V |
| $\Phi_0$ | Onset potential of SEI formation vs. $Li/Li^+$[4] | 800 / fit | mV |
| $D_{EC}$ | Diffusion coefficient of EC in SEI pores | fit | $m^2\,s^{-1}$ |
| $\kappa$ | SEI conductivity | fit | $S\,m^{-1}$ |
| $D_{Li_I}$ | Diffusion coefficient of $Li_I$ in the SEI | $1.0 \cdot 10^{-15}$ | $m^2\,s^{-1}$ |
| $c_{Li_I,0}$ | $Li_I$ concentration at 0 V vs $Li/Li^+$ | fit | $mol\,m^{-3}$ |
| $L$ | SEI thickness | fit | m |
| $L_0$ | Initial SEI thickness (at $t = 0$) | 15.00 | nm |
| $V$ | Partial molar volume of the SEI (LiEDC)[6] | 95.86 | $\mu m^3\,mol^{-1}$ |
| $s$ | Stoichiometric coefficient of EC, $e^-$ or $Li_I$ in the SEI formation reaction (SI-8)[3] | 2 | - |
| $A/A^*$ | Surface area of the negative electrode | 14.34 | $m^2$ |
| $Q_0$ | Nominal cell capacity[7] | 10080 | C |
| $Q_{actual}$ | $= Q_0 - Q_{irr}$, cell capacity during storage | | C |
| $Q_{irr}$ | $= Q_{irr}^{lin} + Q_{irr}^{SEI}$, total capacity irreversibly lost during the storage experiment (zero at $t = 0$) | | C |
| $Q_{irr}^{lin}$ | Capacity lost to SEI cracking, delamination and regrowth | | C |

| | | | |
|---|---|---|---|
| $Q_{\mathrm{irr}}^{\mathrm{SEI}}$ | Capacity lost to SEI formation during the storage experiment (zero at $t = 0$) | | C |
| $Q_{\mathrm{irr},0}^{\mathrm{SEI}}$ | Capacity consumed by SEI formation before experiment (corresponds to SEI thickness $L_0$) | | C |
| $j_{\mathrm{SEI}}^{(i)}$ | Flux density of SEI precursor ($i$) towards the reaction interface | | $\mathrm{C\,s^{-1}\,m^{-1}}$ |
| $\gamma$ | $= \partial_t Q_{\mathrm{irr}}$ | 18.80 | $\mu\mathrm{C\,s^{-1}}$ |
| RC | Relative capacity, relative to $Q_0$ | | % |
| SoC | Full cell state of charge relative to $Q_0$ | | % |
| $t$ | Time measured from the beginning of the storage experiment | | s |
| $t_k$ | Time at which the $k$-th checkup is performed | | s |
| $\tau$ | Constant determined by evaluating eq. (6) at $t = 0$ | | s |
| $\mu_{\mathrm{Li}_x\mathrm{C}_6}^{\mathrm{Li}}$ | Electrochemical potential of lithium in carbon at $x$ SoC | | $\mathrm{J\,mol^{-1}}$ |
| $\mu_{\mathrm{SEI}}^{\mathrm{Li_I}}$ | Electrochemical potential of a neutral lithium interstitial in the SEI host lattice | | $\mathrm{J\,mol^{-1}}$ |
| $\mu_{\mathrm{SEI},0}^{\mathrm{Li_I}}$ | Electrochemical potential of a neutral lithium interstitial in the SEI host lattice at 0 V vs. $\mathrm{Li/Li^+}$ | | $\mathrm{J\,mol^{-1}}$ |
| $F$ | Faraday constant | 96485 | $\mathrm{C\,mol^{-1}}$ |
| $R$ | Gas constant | 8.314 | $\mathrm{J\,mol^{-1}\,K^{-1}}$ |
| $T$ | Temperature (50°C) | 323.15 | K |
| $e$ | Elementary charge | $1.602 \cdot 10^{-16}$ | C |

TABLE SI-2: List of parameters and variables. Note that parameters labeled “fit” are listed in table SI-1.

* Corresponding author: birger.horstmann@dlr.de

[1] Li, D.; Danilov, D.; Zhang, Z.; Chen, H.; Yang, Y.; Notten, P. H. L. *Journal of the Electrochemical Society* **2015**, *162*, A858–A869.

[2] Keil, P. Aging of Lithium-Ion Batteries in Electric Vehicles. PhD Thesis, Technische Universität München, München, 2017.

(3) Zhuang, G. V.; Xu, K.; Yang, H.; Jow, T. R.; Ross, P. N. *The Journal of Physical Chemistry B* **2005**, *109*, 17567–17573.

(4) Edström, K.; Herstedt, M.; Abraham, D. P. *Journal of Power Sources* **2006**, *153*, 380–384.

(5) Kulova, T.; Skundin, A.; Nizhnikovskii, E.; Fesenko, A. *Russian Journal of Electrochemistry* **2006**, *42*, 259–262.

(6) Borodin, O.; Smith, G. D.; Fan, P. *The Journal of Physical Chemistry B* **2006**, *110*, 22773–22779.

(7) Keil, P.; Schuster, S. F.; Wilhelm, J.; Travi, J.; Hauser, A.; Karl, R. C.; Jossen, A. *Journal of The Electrochemical Society* **2016**, *163*, A1872–A1880.
